# Supplementary material for: Which Channel to Ask My Question? Personalized Customer Service Request Stream Routing using Deep Reinforcement Learning
Source: arXiv:1911.10521 source file (2019-11-24)
Supplement: Supplementary file 1 [file appendix.tex]

\begin{appendices}
\section{}
\label{appendices-reward}
Suppose there are three communication channels($n = 3$)
\begin{equation*}
    \begin{split}
        s &= \langle{u, \hat{e}_t, c}\rangle \\
    &= \langle{[0.685, 0.331, 1.0],[5000,5000,88],[128,60,364]}\rangle
    \end{split}
\end{equation*}

where (i)$u = [0.6848884, 0.33148158, 1.0]$ shows the customer's acceptance probability
of three communication channels are 0.6848884, 0.33148158 and 1.0 respectively;
(ii)$\hat{e}_t = [128,60,364]$ shows the channels’ future request flow is 128,60,364 respectively;
(iii)$c = [500,500,88]$ shows the the three communication channels’ capacity is 500,500,88 respectively.

The function of reward is as eq\ref{reward-function}:

\begin{equation}
\label{reward-function}
  \begin{split}
  R=g_{a, t}&-\lambda_1 \cdot \var{ReLu}\left(-\min(\mathbf{c}_{t}-\lambda_3\cdot\hat{\mathbf{e}}_{t+1} )\right) \\
  &-\lambda_2\cdot (\var{ReLu}(\min(\mathbf{c}_{t} - \lambda_3\cdot\hat{\mathbf{e}}_{t+1} )))^2.
  % \mbox{s.t.}\, \lambda_1 \gg 
  %\lambda_2.
  \end{split}
\end{equation}

The calculation process of reward is as follows:
\begin{enumerate}
    \item set $\lambda_1 = 0.5,\lambda_2 = 0.015, \lambda_3 = 0.3$
    \item $\mathbf{c}_{t}-\lambda_3\cdot\hat{\mathbf{e}}_{t+1} = [500,500,88] - 0.3 \times [128,60,364] = [461.6,482,-21.2]$
    \item $min(\mathbf{c}_{t}-\lambda_3\cdot\hat{\mathbf{e}}_{t+1}) = -21.2$
    \item $ Relu(-min(\mathbf{c}_{t}-\lambda_3\cdot\hat{\mathbf{e}}_{t+1})) = 6.36$
    \item if the system recommendes the first communication channels for the customer 
    \begin{itemize}
        \item if the customer accepts the recommendation, then $g_{a,t} = 1$
        \item if the customer rejects the recommendation, then $g_{a,t} = 0$
    \end{itemize}
    \item We assume that the customer accepts the recommendataion, $g_{a,t} = 1$
    \item $R = g_{a,t} - \lambda_1 \times 6.36 - \lambda_2 \times 6.36^2 = 1 - 0.5 \times 6.36 - 0.015 \times 6.36^2 \approx -2.787 $
    
\end{enumerate}

\end{appendices}
